# Supplementary material for: Time Series Data Augmentation for Deep Learning: A Survey
Source: arXiv:2002.12478 source file (2022-03-31)
Supplement: Supplementary file 1 [file 8_Appendix.tex]

\section{Appendix: Data Augmentation}\label{subsec:data-aug}

Data augmentation~\cite{deep:learning:book}, which generates artificial data for training, is an effective way to improve performance in deep learning, especially when the amount of the training data is limited. Currently, very few work has been done on data augmentation for time series data~\cite{data:aug:tsc:2018,Um:data:aug}. Note that the labeled data in time series anomaly detection is generally very limited. In this subsection, we present several practical and effective data augmentation techniques specifically designed for time series after our robust decomposition, in both time domain and frequency domain.  

\subsubsection{Time Domain}

We summarize several effective transforms for time series anomaly detection in the time domain, including flipping, downsampling, cropping, and label expansion, etc. The augmented time series have been plotted in Figure~\ref{fig:time_domain_augmetation}. In the following discussion, we assume we have an input time series $x_1, \cdots, x_N$.  

\textit{Flipping.} We generate a new sequence $x^{'}_1, \cdots, x^{'}_N$ where $x^{'}_t = -x_t$ with the same anomaly labels. It can be used when we care anomalies in both directions. In the scenarios where we are interested in only one direction, this transform cannot be applied. 

% For an input time series $x_1, \cdots, x_n$, we can obtain its opposite numbers $y_t = -x_t$. This upside-down transform doesn't change the label, since we assume that both up and down directions share the same sensitivity to anomalies. 

\textit{Downsampling.} We down sample the original time series of length $N$ with a specific down sample rate $k$, to get a shorter time series with length $\lfloor N/k\rfloor$. 
The label series are also down sampled, or diluted, in the same rate $k$ as values series.

We have tried to duplicate and concatenate $k$ number of those shorter time series to form a new time series with the same length $N$ as the original time series. However, this method does not work well since the connecting points are usually big jumps and they break the time dependencies of time series.

% In this method, We down sample the original time series with length $L$ with a specific down sample rate $k$, to get a shorter time series with length $L/k$. Then we duplicate and concatenate $k$ number of those shorter time series to form a new time series with the same length $L$ as the original time series. 

% The label series are also be down sampled and duplicated the same as values series. The anomalies are diluted, then duplicated. In other words, the label will be kept along with the points that associated with anomalies in the original time series. Here We assume that the anomalies does not change when we scale, zoom in or out the time series. (Need Images)

\textit{Cropping.} We crop samples with replacement from the original time series of length $N$ to get shorter time series with length $N'$. The label series are also cropped, with the same time stamp as values series. This is similar to random crop in computer vision. 

\textit{Label Expansion.} In time series anomaly detection, the anomalies generally occur sequentially. As a result, a data point which is close to a labeled anomaly in terms of both time distance and value distance is very likely to be an anomaly. We select those data points and label as anomalies in our training dataset. 

% We observed that the anomalies usually cluster together in open data sets and rear world scenarios. And it that this can be treated as one last-for-period.

%%\textit{Other methods.} In our study we also tested other transforms for data augmentation in time domain. Unfortunately, they do not lead to performance improvement in our empirical studies, including: 1) During down sampling and cropping, the generated time series have fixed length. However, we also tried to generate variable lengths of time series among mini-batches and feed them to the network for training. Although we keep the length fixed within same mini-batch, it still seems to confuse the network and the results are negative. 2) Other typical time series augmentations such as affine, random jitters, cross sum, etc., which listed in \footnote{https://github.com/terryum/Data-Augmentation-For-Wearable-Sensor-Data} \footnote{https://github.com/arundo/tsaug} \footnote{https://github.com/hfawaz/aaltd18} are also neutral, as they hardly preserve the relation between values and labels.

\begin{figure}[!htb]
    \centering
    \includegraphics[width=\linewidth]{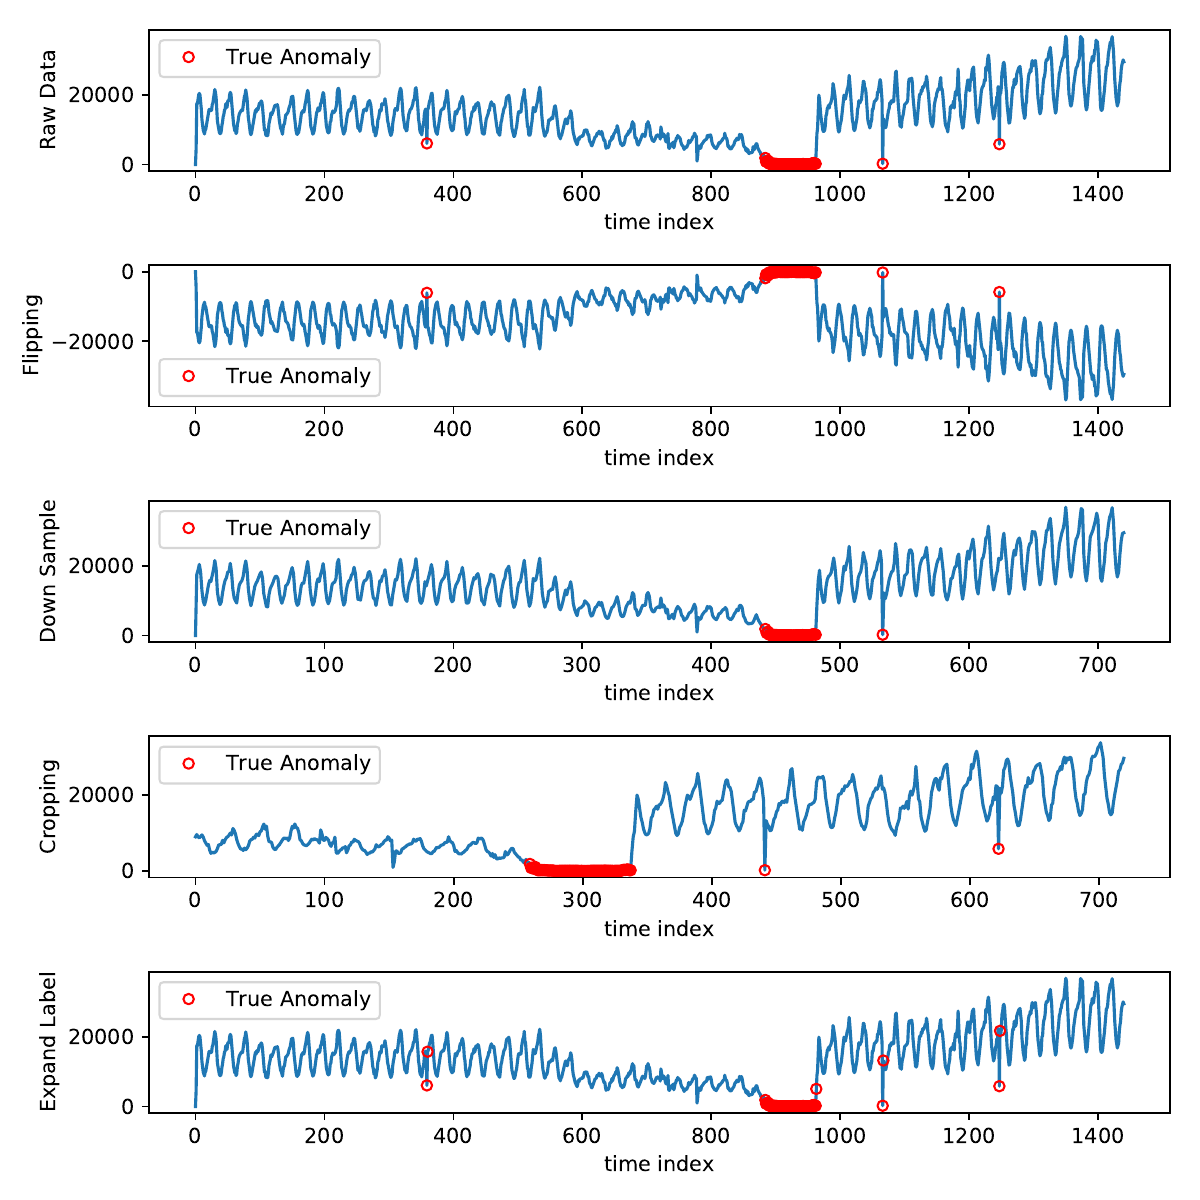}
    \caption{Plots of time series using time domain augmentations. The down sample rate is 2 and cropping length is half of the raw data length.}
    \label{fig:time_domain_augmetation}
\end{figure}

% \vspace{-0.4cm}

\subsubsection{Frequency Domain}

% For a input time series of length $N$, we can obtain its amplitude spectrum and phase spectrum, whose length is $N' = \Bigl\lceil \frac{1}{N} \Bigr\rceil$. Specifically, the amplitude spectrum and phase spectrum are calculated as:

To further increase the labeled data and utilize the special properties of time series data, we explore the data augmentation methods in the frequency domain. Specifically, we have developed several different policies, i.e., magnitude augmentation and phase augmentation, to generate more artificial labeled data. 

% While most existing efforts for time series data augmentation focus on time domain, we instead explore the frequency spectrum and demonstrate that...
% we have chosen the following deformations to make up a augmentation policy

For the input time series $x_1, \cdots, x_N$, we can get its frequency spectrum $F(\omega_k)$ through discrete Fourier transform as follows: 
\begin{equation*}
F(\omega_k) \!=\! \frac{1}{{N}} \!\!\sum_{t=0}^{N-1} \! x_te^{-j\omega_k t}\!=\!\Re[F(\omega_k)] + j\Im[F(\omega_k)], ~ k\!=\!0,1,\!\cdots\!, N\!-\!1
\end{equation*}
where $\Re[F(\omega_k)]$ and $\Im[F(\omega_k)]$ are the real and imaginary parts of the spectrum respectively, and $\omega_k= \frac{2\pi k}{N}$ is the angular frequency. Since $F(\omega_k)$ is complex valued, a more informative representation can be obtained by its amplitude and phase spectra~\cite{BLACKLEDGET200675}:
\begin{equation*}
F(\omega_k) = A(\omega_k) \exp[j\theta(\omega_k)],
\end{equation*}
where $A(\omega_k)$ is the amplitude spectrum defined as
\begin{equation*}
A(\omega_k)=|F(\omega_k)|=\sqrt{\Re^2[F(\omega_k)] + \Im^2[F(\omega_k)]},
\end{equation*}
and $\theta(\omega_k)$ is the phase spectrum defined as 
\begin{equation*}
\theta(\omega_k)=\tan^{-1}\frac{\Im[F(\omega_k)]}{\Re[F(\omega_k)]}.
\end{equation*}
Note that the input time series is real signal, the length of amplitude and phase spectra is $N' = \Bigl\lceil \frac{N+1}{2} \Bigr\rceil$.

In the frequency domain, our intuitive idea is to make perturbations in magnitude and phase in selected segments in the frequency domain. We define the selected segment length $K$ by the ratio $r$:
$$
K=rN'.
$$
Let define the number of segments as $m_K$. Then, each segment with starting point as $k_i$ in frequency domain is obtained as:
$$
[k_i, k_i + K), ~\text{where}~ k_i \sim U(0, N'-K), ~ i=1,2,\cdots, m_K.
$$
Here we also ensure that the overlapping part of consecutive segments is not exceeding the half length of segment length $K$, i.e., 
$$
|k_i-k_{i+1}|\geq \frac{K}{2}, ~  i=1,2,\cdots, m_K-1.
$$

In magnitude augmentation, we make perturbations in the magnitude spectrum. Specifically, we replace the values of all points in the selected segment with $\upsilon$, where $\upsilon$ has Gaussian distribution as $\upsilon  \sim N(\mu_A,q_A \bar{\delta}^2_A)$,
% $$
% \upsilon  \sim N(\mu_A,q\delta^2_A), ~\text{or}~\upsilon  \sim N(0,q_A\delta^2_A)
% $$
where $\mu_A$ can be set as zero or $\bar{\mu}_A$ based on configuration, and $\bar{\mu_A}, \bar{\delta}^2_A$ is the sample mean and variance of the time series in the segment, respectively, and $q_A$ is adopted to control the degree of perturbation.

Similarly, we can make perturbation in the phase spectrum in phase augmentation. Specifically, the values of all points in the selected segment are increased by a small perturbation $\theta$, which is sampled from Gaussian distribution as
$\theta \sim N(0,\delta_{\theta}^2)$.

The proposed frequency-domain time series augmentation methods on a sample data is plotted in Figure~\ref{fig:3-freqAugDemo} for illustration.
\begin{figure}[]
    \centering
    \includegraphics[width=1\linewidth]{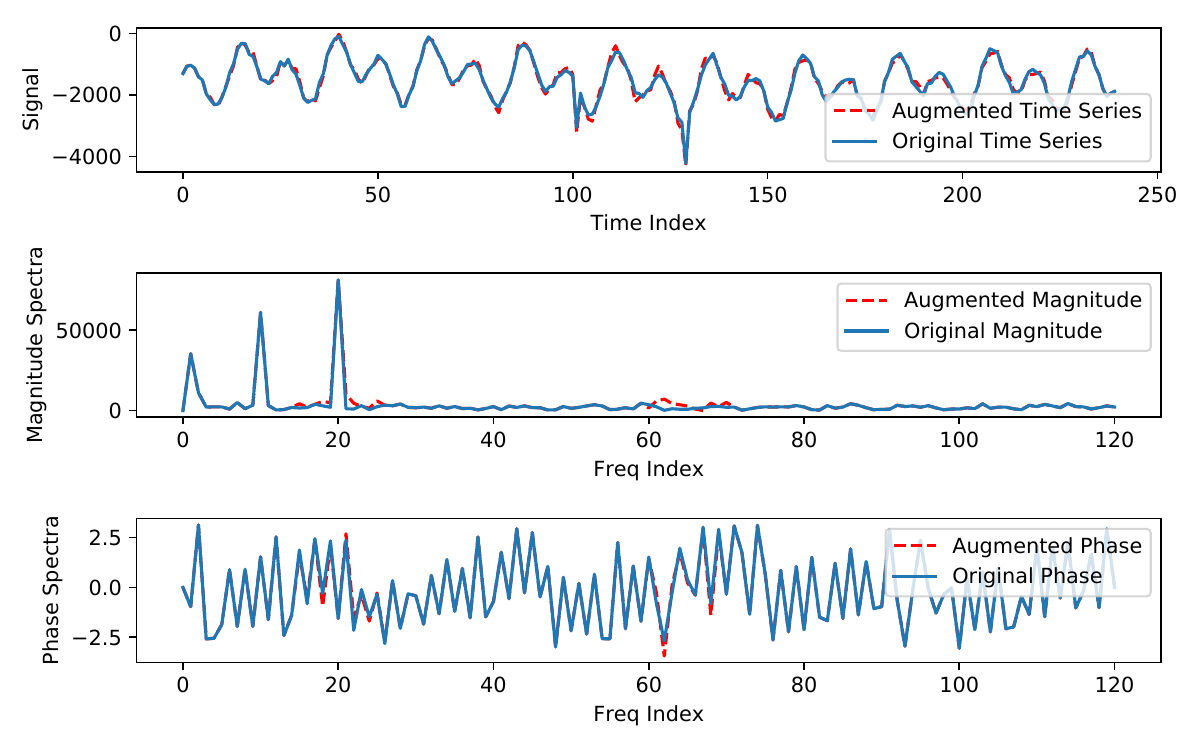}
    \caption{Plots of time series using magnitude augmentation and phase
    augmentation.}
    \label{fig:3-freqAugDemo}
\end{figure}
% \vspace{-0.3cm}

% \begin{comment}
We have performed extensive empirical studies on different time series datasets. Table~\ref{tab:3-freqAugPolicy} summarizes the recommended parameter settings for magnitude augmentation and phase augmentation in the frequency domain. 
\begin{table}[]
    \centering
        \caption{Frequency domain augmentation parameter recommendation for magnitude augmentation and phase 
        augmentation.}
\begin{tabular}{c|ccccc}
\hline
{Policy} &  $r$ &  $m_K$ &  $\mu_A$ & $q_A$& $\delta_{\theta}^2$  \\
\hline
None    &  0    & 0 &  -    & -   &  -   \\
Basic   &  0.05 & 2 & 0  & 0.1 &  0.1 \\
Strong  &  0.1  & 3 & $\bar{\mu}_A$  & 0.2 &  0.2 \\
\hline
\end{tabular}
    \label{tab:3-freqAugPolicy}
\end{table}
% \end{comment}

% ts: 240 length. [20., 10.] peak --> periods: 12 .  24 . （outlier）  101,129,
